# Supplementary material for: Sim-to-Real Transfer for Biped Locomotion
Source: arXiv:1903.01390 source file (2019-08-25)
Supplement: Supplementary file 1 [file appendix.tex]

\section*{APPENDIX}
\karen{Condense this into one paragraph in Experiements section.}
In this appendix, we detail the generic motion trajectories we design for pre-sysID stage. Specifically, we design two types of motion trajectories: joint exercise motions and stand/falling motions.

In the first class of trajectories, we apply a step function to each motor on the robot, starting from a random pose. One such example can be seen in Figure \ref{fig:sysid_comp}. We use step functions of magnitude $0.1$, $0.3$ and $0.6$ to collect motor behaviors at different speed. We generate these trajectories automatically in simulation, such that no self-collision is allowed. When collecting trajectories of the first category, we manually hold the robot torso, such that the feet do not collide with the ground.

In the second class of trajectories, we collect data that involves ground contact. We first create a squat and stand pose and linearly interpolate them to produce a stand-up trajectory. We collect three stand-up sequences with different interpolation speed, where in all three trajectories the robot does not lose balance. In addition, we script three motions, where the robot falls forward, sideways and backward. 

For all trajectories, we collect the motor position and the estimated orientation from the IMU sensor for simulation parameter optimization.
